# Supplementary material for: The Effect of Behavioral Probability Weighting in a Simultaneous Multi-Target Attacker-Defender Game
Source: arXiv:2103.03392 source file (2021-03-05)
Supplement: Supplementary file 1 [file Appendix.tex]

\subsection{Effect of Probability Weighting on Investments}
Now, we compare the investments of behavioral defender with the investments of the non-behavioral defender.%\footnote{One can also consider a behavioral attacker; however, in this paper, we focus only on behavioral decision-making by the defender in order to better understand its impact on the game, and leave the consideration of a behavioral attacker for future work.} 

\begin{proposition}\label{prop:behavioral-suboptimal}
Consider a non-behavioral attacker $\mathcal{A}$ (i.e., $\alpha_{\mathcal{A}} = 1$) and a behavioral defender $\mathcal{D}$ (i.e., $\alpha_{\mathcal{D}} < 1$). Let the true probability of successful attack on each asset be given by \eqref{eq: defend-attack expon probability}. Consider a set of $n$ assets whose gains can be put in descending order $G_{1} \geq G_{2} \geq  \dots \geq  G_n$ such that $\frac{G_i}{G_j} \geq \frac{L_i}{L_j} \enspace \forall i < j$.  Suppose that the pre-existing defense investments on each asset satisfy $a_1 = a_2 = \dots = a_n$. Then, the investment profile of non-behavioral defender (in Proposition~\ref{prop: optimal attack allocation ordered}) is not optimal from the perspective of a behavioral defender. 
\end{proposition}

\begin{proof}
By Proposition~\ref{prop: optimal attack allocation ordered}, it is optimal for a non-behavioral defender to invest the entire budget on the nodes such that the relation between any two nodes $v_i$ and $v_j$ with nonzero optimal investment is given by
$$
x_i^* = x_j^* + \log(\frac{L_i}{L_j})
$$ 
in order to minimize the cost function \eqref{eq: defender rational cost node}. Now, we will show that this investment is not optimal with respect to the behavioral defender's perceived cost function \eqref{eq: defender cost node} where she can decrease her cost by deviating from $\mathbf{x}^*$ via moving  sufficiently small investment from an asset with lower loss valuation and has nonzero optimal investment, denoted by $v_j$ to the first asset $v_1$ with the highest loss valuation contradicting the fact that $\mathbf{x}^*$ is a PNE investment for the behavioral defender.

Starting with the optimal investments of the rational (non-behavioral) defender (as given by Proposition~\ref{prop: optimal attack allocation ordered}), if the probability of successful attack on each asset is given by \eqref{eq: defend-attack expon probability}, the behavioral defender's perceived cost in \eqref{eq: defender cost node} will be:
\begin{align*}
C_{\mathcal{D}}(\mathbf{x}^*,\mathbf{y}) &=  \sum_{i=1}^{n} L_i \hspace{1mm} w_{\mathcal{D}}(p_i(x_i^*, y_i)).
\end{align*}
%% \iffalse &\stackrel{(a)}= L_{1} \hspace{1mm} L_1 \hspace{1mm} w_{\mathcal{D}}(p_1(x_1^*, y_i)) \\ &+ L_j \hspace{1mm} e^{-\left(x_1 + \log(\frac{L_j}{L_1}) - \log(1 - e^{\gamma_j+\log(\frac{L_j}{L_1})})\right)^{\alpha_{\mathcal{D}}}}  \\ &+  \underset{i \neq j}{\sum_{i=2}^{n}} L_i \hspace{1mm} e^{-\left(x_i - \log(1 - e^{-y_i})\right)^{\alpha_{\mathcal{D}}}}.
%where (a) holds from the non-behavioral attacker's optimal investments from Proposition~\ref{prop: optimal attack allocation ordered} and $\gamma_i = - (y_j + \log(\frac{G_i}{G_j}))$ and from the relation $x_1 = x_j + \log(\frac{L_1}{L_j})$ between the nodes $v_1$ and $v_j$.

Now, remove a small investment $\epsilon$ from the node $v_j$, and add an investment of $\epsilon$ to the first node $v_1$. Denote the modified investment vector by $\bar{\mathbf{x}}$.  The perceived cost in \eqref{eq: defender cost node} under this investment vector will be
\begin{multline*}
C_{\mathcal{D}}(\bar{\mathbf{x}},\mathbf{y}) =  L_1 \hspace{1mm} w_{\mathcal{D}}(p_1(x_1^*+\epsilon, y_1)) + L_j \hspace{1mm} w_{\mathcal{D}}(p_j(x_j^* - \epsilon, y_j)) \\ + 
  {\sum_{i\notin \{1,j\}}} L_i \hspace{1mm} w_{\mathcal{D}}(p_i(x_i^*, y_i)).
\end{multline*}
The net reduction in the perceived cost will be positive if 
$C_{\mathcal{D}}(\bar{\mathbf{x}},\mathbf{y}) < C_{\mathcal{D}}(\mathbf{x}^*,\mathbf{y})$. Define
\begin{equation*}
f(\epsilon) =  L_1 \hspace{1mm} w_{\mathcal{D}}(p_1(x_1^*+\epsilon, y_1)) + L_j \hspace{1mm} w_{\mathcal{D}}(p_j(x_j^* - \epsilon, y_j)) .
\end{equation*}
and note that
\begin{align*}
    C_{\mathcal{D}}(\mathbf{x}^*, \mathbf{y}) &= f(0) +   {\sum_{i\notin \{1,j\}}} L_i \hspace{1mm} w_{\mathcal{D}}(p_i(x_i^*, y_i)).\\
    C_{\mathcal{D}}(\bar{\mathbf{x}}, \mathbf{y}) &= f(\epsilon) +   {\sum_{i\notin \{1,j\}}} L_i \hspace{1mm} w_{\mathcal{D}}(p_i(x_i^*, y_i)).
\end{align*}  
Thus, $C_{\mathcal{D}}(\bar{\mathbf{x}}, \mathbf{y})$ will be smaller than $C_{\mathcal{D}}(\mathbf{x}^*, \mathbf{y})$ if $f(\epsilon) < f(0)$. 

We have
\begin{align*}
\frac{df}{d\epsilon} &= \left.L_1\frac{\partial w_{\mathcal{D}}(p_1(x,y_1^*))}{\partial x}\right|_{x = x_1^*+\epsilon} -\left.L_j\frac{\partial w_{\mathcal{D}}(p_j(x,y_j^*))}{\partial x}\right|_{x = x_j^*-\epsilon}\\
&= \alpha_{\mathcal{D}}\left[L_j \frac{e^{-(x_j^* - \epsilon +  k_j)^{\alpha_{\mathcal{D}}}}}{(x_j^* - \epsilon + k_j)^{1-\alpha_{\mathcal{D}}}}- L_1\frac{e^{-(x_1^* + \epsilon + k_1)^{\alpha_{\mathcal{D}}}}}{(x_1^* + \epsilon +  k_1)^{1-\alpha_{\mathcal{D}}}}\right].
\end{align*}
\iffalse
For any $\epsilon > 0$, we have
\begin{align*}
\epsilon > 0 
\iff & e^{\gamma_1 + x_1 - x_j + 2\epsilon} > e^{\gamma_1 + x_1 - x_j}\\
\iff &  1 - e^{\gamma_1 + x_1 - x_j + 2 \epsilon} < 1 - e^{\gamma_1 + x_1 - x_j} \\
\iff &-\log(1 - e^{\gamma_1 + x_1 - x_j + 2 \epsilon}) > -\log(1 - e^{\gamma_1 + x_1 - x_j}) \\
\iff & x_1 + \epsilon - \log(1 - e^{\gamma_1 + x_1 - x_j + 2 \epsilon})  \\ & > x_1 -\log(1 - e^{\gamma_1 + x_1 - x_j})\\
\iff & f_1(\epsilon) < f_1(0).
\end{align*}
\fi
Choosing the asset $v_j$ with $k_j - k_1 > \log(\frac{L_1}{L_j}) + 2\epsilon$ (i.e.,  choosing the asset $v_j$ with the lowest attack investment) yields
\begin{align*}
k_j - k_1 > \log(\frac{L_1}{L_j}) + 2\epsilon
\\ \iff & k_j - k_1 > x_1^* - x_j^* + 2 \epsilon\\
\iff & x_j^* + k_j > x_1^* + k_1   + 2 \epsilon \\
\iff & x_j^* - \epsilon + k_j > x_1^* + k_1   + \epsilon.
\end{align*}
Since $\frac{e^{-r^{\alpha_{\mathcal{D}}}}}{r^{1-\alpha_{\mathcal{D}}}}$ is a decreasing function of $r \in (0, \infty)$, this ensures that $\displaystyle \lim_{\epsilon \downarrow 0}\frac{df}{d\epsilon}$ is negative, which shows that $f(\epsilon)$ is decreasing for sufficiently small $\epsilon$. Therefore, $ C_{\mathcal{D}}(\bar{\mathbf{x}},\mathbf{y}) < C_{\mathcal{D}}(\mathbf{x}^*,\mathbf{y})$ for sufficiently small $\epsilon$ (i.e., the defense investment profile $\bar{\mathbf{x}}$ outperforms the investment profile $\mathbf{x}^*$), thereby contradicting the optimality of the investment profile $\mathbf{x}^*$ from the perspective of behavioral defender.
\end{proof}

The above result shows that for a   behavioral defender (specifically, with  nonlinear probability weighting), shifting investments from asset(s) with lower loss valuation to the asset with the highest loss valuation is better for the behavioral defender (i.e., decreases her cost) than the investment profile of the rational defender (presented in Proposition~\ref{prop: optimal attack allocation ordered}). Note that the previous result does not give the optimal investment of the behavioral defender.
